# Supplementary material for: Light Dark Matter Search with Ionization Signals in XENON1T
Source: arXiv:1907.11485 source file (2019-12-17)
Supplement: Supplementary file 1 [file supplement_only_prl.tex]

%%%
% File to produce the supplemental material separately.
% Compiling this files requires main.aux to be present.
% While this is created automatically when main.tex is compiled,
% it is included in the submission for convenience.
%%%

\input{header.tex}

% Allow references to main paper
\usepackage{xr}
\externaldocument{main}

% Allow citing of main paper's bibliography
\usepackage{xcite}
\externalcitedocument{main}

\begin{document}

% Start figures at 6, not 1
\setcounter{figure}{5}

\input{_supplement_content.tex}

\end{document}
